# Supplementary material for: StyleCineGAN: Landscape Cinemagraph Generation using a Pre-trained StyleGAN
Source: arXiv:2403.14186 source file (2024-03-21)
Supplement: Supplementary file 1 [file 900_suppl.tex]

\clearpage

\setcounter{page}{1}
\setcounter{section}{0}

\maketitlesupplementary

\section{Implementation Details}

\label{sec:implementation}
In this section, we provide details about the implementation of our method. Specifically, we explain each component of our method in detail, and provide training details about our encoder network, motion generator, and mask predictor.

\subsection{Detailed explanations of each component}

\paragraph{Mask Prediction}
We first predict the mask using an ensemble of 10 MLP classifiers~\cite{zhang2021datasetgan}, and refine it at inference to further improve the quality.
To accomplish this, we compute contour areas in the mask using a contour detection algorithm~\cite{SUZUKI198532}. Next, each area is considered to be holes and are removed if the ratio of its area with respect to the total area is less than 3$\%$.
This process effectively removes the noise from the predicted segmentation mask $S$ as illustrated in Fig~\ref{fig:seg} (c).

\vspace{-0.2cm}

\paragraph{Multi-Scale Deep Feature Warping}
We warp multi-scale features $D^{i}_{t}$, each of which corresponds to a different resolution. Given that the computed displacement fields $F_{0\to t}$ and $F_{N\to t}$ are at a fixed resolution of 512$\times$512, it is necessary to resize them to match the dimensions of the respective deep features. This resizing operation is carried out using bilinear interpolation. Because the displacement fields represent pixel-level shifts, the values must be adjusted relative to the size of the features they are applied to. For instance, a 2-pixel shift at 256$\times$256 resolution is equivalent to a movement twice the size of a 2-pixel shift at 512$\times$512 resolution. To resolve this scaling discrepancy, we multiply scaling factors $C_{u}$ and $C_{v}$ to the $u$ and $v$ components of the displacement fields, respectively. The scaling factors are defined as $C_{u} = \frac{W}{512}$ and $C_{v} = \frac{H}{512}$, where $W$ and $H$ represent the width and height of the deep feature $D^{i}_{t}$.

\vspace{-0.2cm}

\paragraph{Cinemagraph Generation}
While the multi-scale features warped with modified joint splatting cover most of the pixels, there can be some pixels with missing values. We apply a median filter to $D^{i}_{t}$ to fill these small regions. Our final composited features $D^{i}_{t}$ with missing values filled can be expressed as follows:
\begin{equation}
D^{i}_{t}(x') = (1-H) \odot D^{i}_{t}(x') + H \odot \text{Median}(D^{i}_{t}(x')),
\label{eqn:dfw3}
\end{equation}
where $H$ is a binary hole mask. The mask has a value of 1 for missing pixels and 0 for filled pixels. Median represents a median filter with a kernel of size 7$\times$7. Large holes with more than 3$\%$ of the total area sometimes occur, and in this case a simple image inpainting method~\cite{Telea2004} is applied to $D^{i}_{t}$.

\subsection{Training}

\paragraph{Encoder Network}
To encode an input image into both latent codes and the deep features of StyleGAN, we train an encoder network using the architectures proposed in~\citet{feature-style}. Images from the LHQ~\cite{LHQ} dataset, 84,466 for training and 5,534 for validation, were used to train this encoder network. We trained the network for 12 epochs using the following loss function:
\begin{equation}
    \mathcal{L}_{enc} =  \mathcal{L}_{2} + \lambda_{lpips}\mathcal{L}_{lpips} + \lambda_{reg}\mathcal{L}_{reg},
\label{loss:enc}
\end{equation}
where $\mathcal{L}_{2}$, $\mathcal{L}_{lpips}$, and $\mathcal{L}_{reg}$ are the reconstruction loss, perceptual loss, and feature regularization loss, respectively. $\lambda_{lpips}$ and $\lambda_{reg}$ are the weights for each loss term. We set $\lambda_{lpips}=0.2$ and  $\lambda_{reg}=0.01$. We used the ADAM~\cite{kingma2017adam} optimizer with an initial learning rate of $10^{-4}$, which resulted in a computation time of about 19 hours on an NVIDIA RTX A5000 GPU with a batch size of 1.

\begin{figure}[t!]
    \centering
    \includegraphics[width=.85\columnwidth]{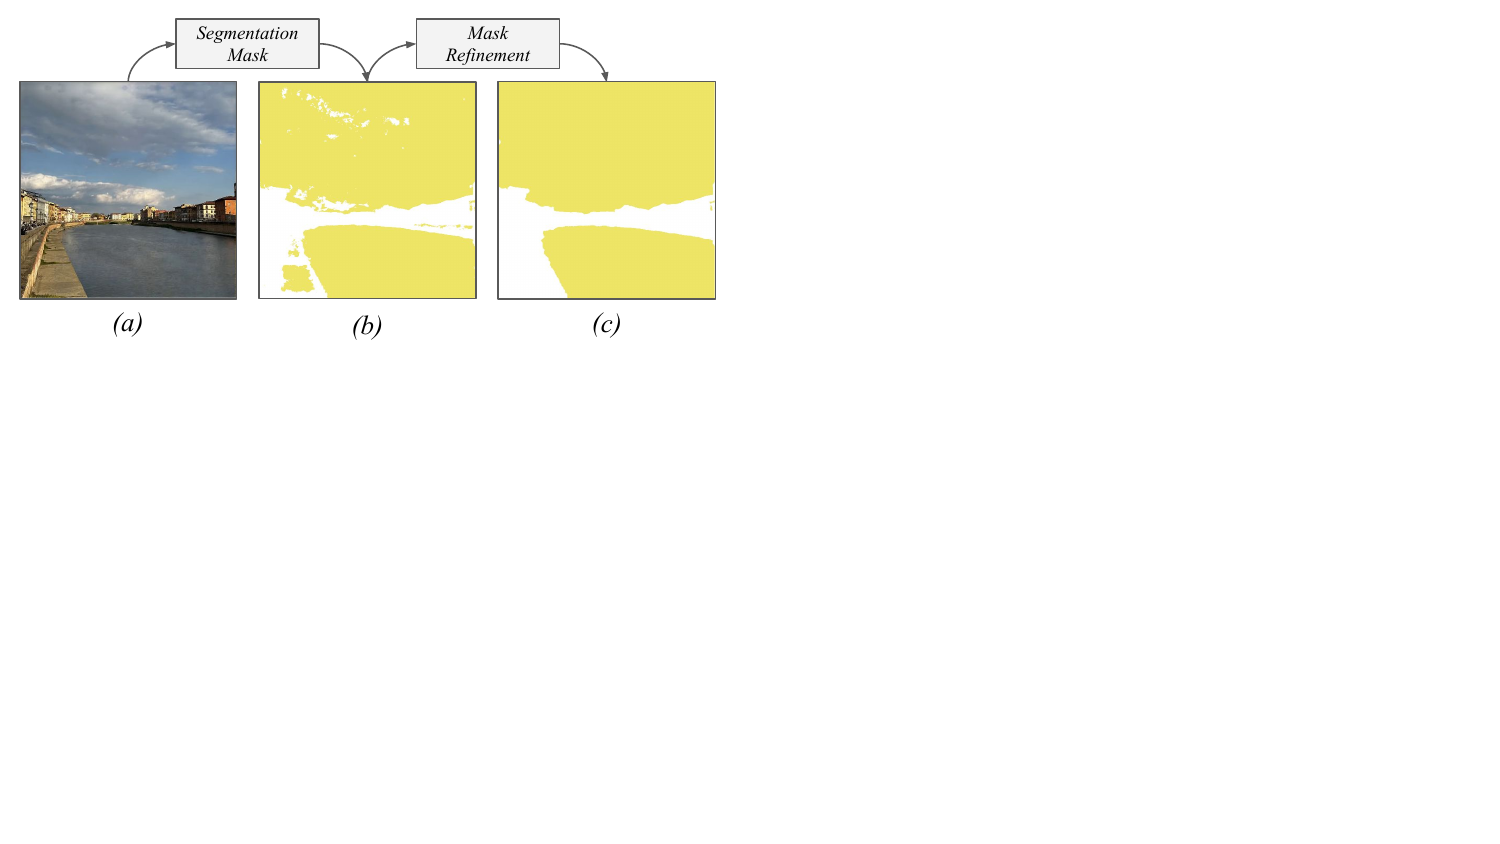}
    \vspace{-0.3cm}
    \caption{Mask prediction results. (a) Given an input image, (b) a mask is predicted by the mask predictor~and~(c) further refined~by~hole~filling.}
    \vspace{-0.45cm}
    \label{fig:seg}
\end{figure}

\vspace{-0.3cm}

\paragraph{Motion Generator}
We trained an image-to-image translation network~\cite{pix2pixHD} as our motion generator. The motion generator was trained for 35 epochs, using the default parameters of \citet{Holynski_2021_CVPR}. For sky motion, a set of 1,060 image-motion pairs from 430 unique videos of Sky Time-Lapse~\cite{Xiong_2018_CVPR} were used for training.
For fluid motion, a set of 4,895 image-motion pairs from 979 unique videos of the Eulerian~\cite{Holynski_2021_CVPR} dataset are used.
We resized all videos to a size of 512$\times$512. To generate ground-truth motion fields, we use a pre-trained optical flow estimator~\cite{RAFT}. The estimator calculates the average optical flow between consecutive frames within a 2-second window.
The motion generator was trained with the ADAM~\cite{kingma2017adam} optimizer with an initial learning rate of $2 \times 10^{-4}$, which resulted in a computation time of about 6 hours on an NVIDIA GeForce RTX 3090 GPU with a batch size of 2.

\paragraph{Mask Predictor}
We trained a MLP classifier as our mask predictor using the architectures proposed in~\citet{zhang2021datasetgan}. An ensemble of 10 MLP classifiers was trained using 32 input features paired with human-annotated segmentation masks. To construct the input feature $D^*$, we first project the annotated images into both $D^{10}$ and $w^{+}$. We then feed $D^{10}$ and $w^{+}$ to a pre-trained StyleGAN to extract the deep features $D^{i}$ where $i \in \{10,11,...,18\}$. These deep features are all resized to 512$\times$512 and concatenated in the channel dimension. The constructed input feature is $D^{*} \in \mathbb{R}^{512\times 512\times 1472}$. We trained each classifier for 3 epochs with the ADAM~\cite{kingma2017adam} optimizer with an initial learning rate of $10^{-3}$. Training all 10 MLP classifiers required about 15 hours of computation time on an NVIDIA Tesla V100 GPU with a batch size of 2.

    % \resizebox{0.8\linewidth}{!}{
    
    %     \begin{tabular}{c|*{9}{c}}\hline
    %     \diaghead{WarpIndexReconIndex}{Warp Index}{Recon Index} & 5 & 6 & 7 & 8 & 9 & 10 & 11 & 12 & 13 \\ \hline
    %     5  & 0.01335                                                      & - & - & - & - & - & - & - & - \\
    %     6  & \textbf{0.01327} & \textbf{0.01324}                               & - & - & - & - & - & - & - \\
    %     7  & 0.0203 & 0.0238 & 0.0128                                            & - & - & - & - & - & - \\
    %     8  & 0.0204 & 0.0239 & \textbf{0.0127}& \textbf{0.0124}                      & - & - & - & - & - \\
    %     9  & 0.0188 & 0.0219 & 0.0210 & 0.0247 & 0.0125                                  & - & - & - & - \\ 
    %     10 & 0.0187 & 0.0219 & 0.0210 & 0.0247 & \textbf{0.0125} & \textbf{0.0124}           & - & - & - \\
    %     11 & 0.0204 & 0.0241 & 0.0236 & 0.0276 & 0.0261 & 0.0271 & 0.0124                        & - & - \\
    %     12 & 0.0205 & 0.0242 & 0.0236 & 0.0276 & 0.0260 & 0.0272 & \textbf{0.0123} & \textbf{0.0122} & - \\
    %     13 & 0.0209 & 0.0232 & 0.0231 & 0.0260 & 0.0253 & 0.0286 & 0.0208 & 0.0275 & 0.0124 \\
    %     14 &  \\
    %     15 \\
    %     16 \\
    %     \end{tabular}

\section{Effectiveness of Deep Feature Warping}
When warping is performed in image space, tearing artifacts are likely to occur for large pixel flows. To evaluate the effectiveness of our method for removing the tearing artifacts, in addition to qualitative and quantitative evaluations, we conducted a human perceptual study. The user study involved 19 participants who were presented with cinemagraph results and asked to score the occurrence of tearing artifacts. The ratings were made on a 1-to-5 scale, with "strongly disagree" being 1 and "strongly agree" being 5. The scores reported in Table~\ref{tab:suppl_dfw} reveal that the application of DFW indeed removes the tearing artifacts, proving its effectiveness.
\begin{table}[]
    \centering
    \caption{Human perceptual study results for assessing the occurrence of tearing artifacts. The best scores are bolded.}

    \vspace{-0.2cm}

    \resizebox{.6\columnwidth}{!}{
    \begin{tabular}{cc}
    \hline
    Method           &  Tearing Artifacts $\downarrow$  \\ \hline
    Ours - w/o DFW   &  4.37 $\pm$ 0.83                 \\
    Ours - Full      &  \textbf{1.97 $\pm$ 0.99}        \\ \hline
    \end{tabular}}

    \vspace{-0.3cm}
    
    \label{tab:suppl_dfw}
\end{table}

\vspace{-0.2cm}

\section{Selection of Deep Feature Index}
Our method utilizes the deep features of a pre-trained StyleGAN for both the GAN inversion and cinemagraph generation process. Various deep features $D^{i}$ where $i \in [1, 2, ..., 18]$ can be obtained from StyleGAN, thus we conducted a series of experiments to determine the proper index for our task.

\subsection{Reconstruction and Warping Index} \label{suppl:recon_warp}
For each GAN inversion and DFW, a different feature index $i$ can be used. Thus we explored various combinations of feature indices to assess which one led to the best perceptual quality. For GAN inversion, we employed feature indices $i \in [5, 6, ..., 13]$, while for DFW, we utilized feature indices $j \in [i, i+1, ..., 16]$. To assess the perceptual quality of the generated cinemagraphs, we measured LPIPS~\cite{zhang2018perceptual} between the generated frame $\hat{I}_n$ and the corresponding ground truth frame $I_n$ using 224 test videos from the Sky Time-Lapse dataset~\cite{Xiong_2018_CVPR}. Table~\ref{tab:suppl_feat_select} reveals the quantitative evaluation results on perceptual quality. The results show that the perceptual quality tends to improve as higher feature indices are employed for reconstruction. The highest perceptual quality is achieved when the latest feature index~$j \in [6, 8, ..., 16]$~within the same StyleGAN block as the reconstruction index $i$ is used for warping. Specifically, pairs $(i, j)$ such as $(5,6), (6, 6), (7, 8), (8, 8), ..., (15, 16),$ and $(16, 16)$ produce the highest perceptual quality for each reconstruction index~$i$.

\subsection{Perceptual Quality and Stylization Ability}
We searched for the sweet spot in a trade-off between perceptual quality and stylization ability. We used 224 test videos from the Sky Time-Lapse dataset~\cite{Xiong_2018_CVPR}, utilizing the feature index pairs $(i,j)$ with the highest perceptual quality described in Sec.~\ref{suppl:recon_warp}.
To assess perceptual quality, we computed LPIPS between the generated frame $\hat{I}_n$ and its corresponding ground-truth frame $I_{n}$. To evaluate stylization ability, we computed RMSE between the Gram matrix~\cite{NeuralTexture} extracted from the target style image $G(w_{t}^{+})$ and the generated frame $G_{warp}(D^{10}, w_{s}^{+}, F_{0\to t}, F_{N\to t})$. Target style latent $w_{t}^{+}$ was obtained from 16 color images from the RYB color model. We optimized $w_{t}^{+}$ while fixing StyleGAN, using the ADAM~\cite{kingma2017adam} optimizer with an initial learning rate of 0.1. Figure~\ref{fig:suppl_feat_idx} shows the trade-off between perceptual quality and stylization ability: when we increase feature index $i$, the generated cinemagraphs exhibit higher perceptual quality but demonstrate less stylization ability. We selected feature index~$i=10$~considering~this~trade-off.

% To measure perceptual quality, we computed LPIPS between generated frame $\hat{I}_n$ and corresponding ground-truth frame $I_n$.
% To measure stylization ability, we computed RMSE between the Gram matrix~\cite{NeuralStyle} extracted from the target style image $G(w_{t}^{+})$ and the generated frame $G_{warp}(D^{10}, w_{s}^{+}, F_{0\to t}, F_{N\to t})$. Figure~\ref{fig:suppl_feat_idx} shows trade-off between perceptual quality and stylization ability: when we increase feature index $i$, the generated cinemagraphs are with higher perceptual quality but with less stylization ability. We choose feature index $i = 10$ considering this trade-off.

% Gram matrix~\cite{NeuralTexture}
% between generated stylized frame $G_{warp}()$

%% Feature Index Table
\begin{table}[t]
\centering

\caption{Quantitative evaluation of perceptual quality according to reconstruction and warping indices. The best scores are bolded.}

\vspace{-0.2cm}

\resizebox{\columnwidth}{!}{
\begin{tabular}{c |*{9}{c}}\hline
     \diaghead{WarpIndexReconIndex}{Warp Index}{Recon Index} & 5 & 6 & 7 & 8 & 9 & 10 & 11 & 12 & 13 \\ \hline
     5  & .01335                                                             & - & - & - & - & - & - & - & - \\
     6  & \textbf{.01327} & \textbf{.01324}                                      & - & - & - & - & - & - & - \\
     7  & .02033 & .02388 & .01284                                                   & - & - & - & - & - & - \\
     8  & .02042 & .02388 & \textbf{.01279} & \textbf{.01265}                            & - & - & - & - & - \\
     9  & .01882 & .02199 & .02105 & .02475 & .01258                                         & - & - & - & - \\
     10 & .01877 & .02199 & .02107 & .02478 & \textbf{.01251} & \textbf{.01246}                  & - & - & - \\
     11 & .02049 & .02418 & .02363 & .02761 & .02612 & .02717 & .01240                               & - & - \\
     12 & .02054 & .02420 & .02362 & .02761 & .02608 & .02729 & \textbf{.01238} & \textbf{.01224}        & - \\
     13 & .02098 & .02324 & .02319 & .02609 & .02535 & .02869 & .02083 & .02759 & .01248                     \\
     14 & .02094 & .02323 & .02319 & .02603 & .02535 & .02676 & .02075 & .02759 & \textbf{.01235}            \\
     15 & .02277 & .02432 & .02429 & .02708 & .02729 & .02859 & .02348 & .02835 & .02533                     \\
     16 & .02322 & .02460 & .02453 & .02731 & .02736 & .02861 & .02360 & .02840 & .02530                     \\
\end{tabular}
}
\label{tab:suppl_feat_select}
\end{table}

\vspace{-0.2cm}

\begin{figure}[t!]
    \centering
    \includegraphics[width=.75\columnwidth]{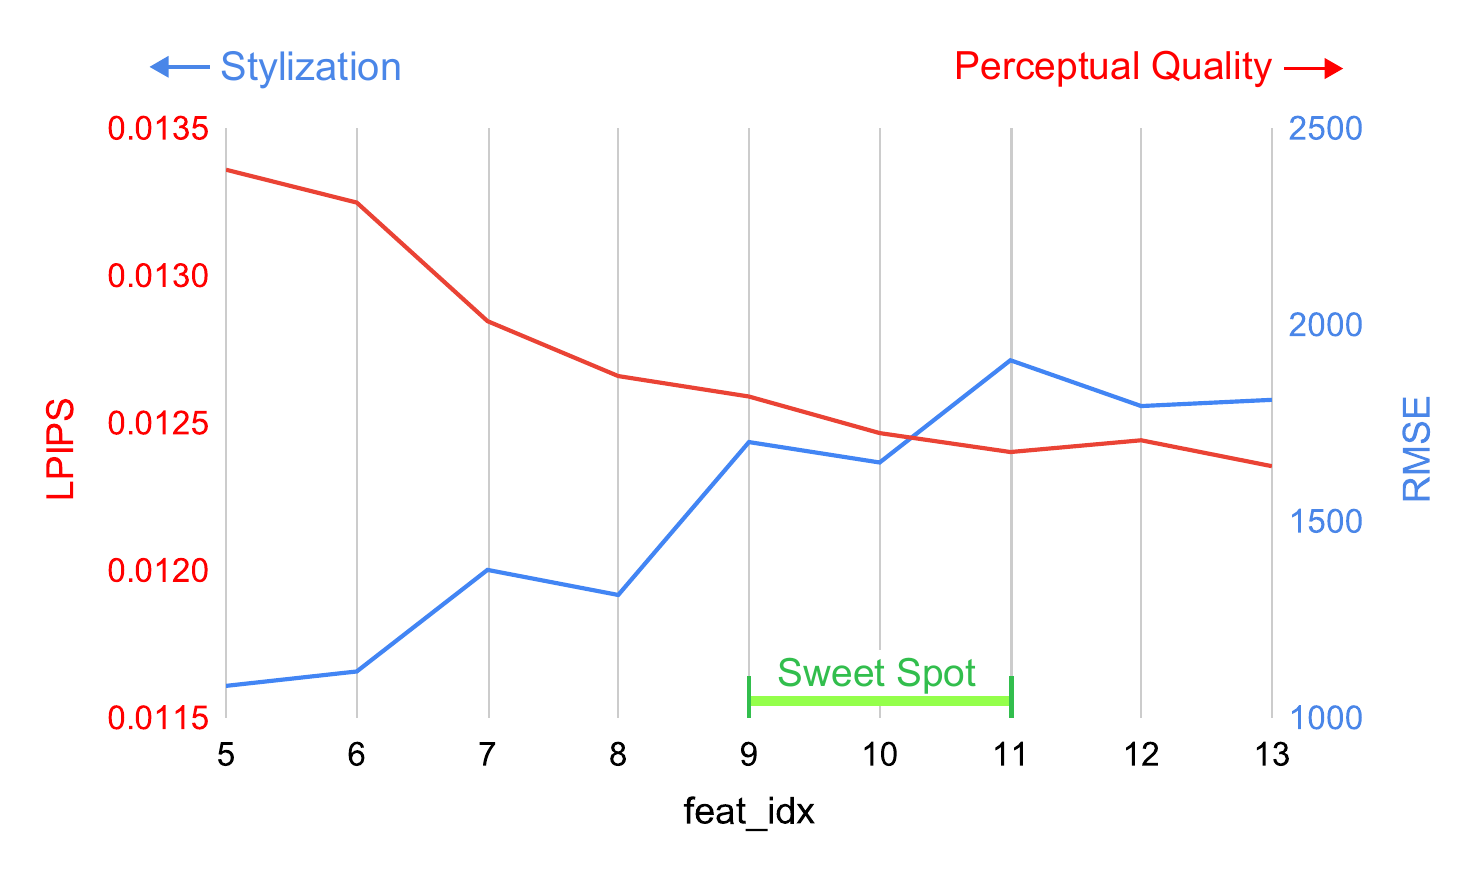}
    \vspace{-0.3cm}
    \caption{Trade-off between perceptual quality and stylization according to feature index $i$.}
    \vspace{-0.3cm}
    
    \label{fig:suppl_feat_idx}
\end{figure}
